# Supplementary material for: Experimental determination of the spin Hamiltonian of the cubic chiral magnet MnSi
Source: arXiv:2401.10687 source file (2024-01-19)
Supplement: Supplementary file 1 [file MnSi_Hamiltonian_SM.pdf]

# Supplemental Material for “Experimental determination of the spin Hamiltonian of the cubic chiral magnet MnSi”

P. Dalmas de Réotier,<sup>1</sup> A. Yaouanc,<sup>1</sup> G. Lapertot,<sup>1</sup> C. Wang,<sup>2</sup> A. Amato,<sup>2</sup> and D. Andreica<sup>3</sup>

<sup>1</sup>*Université Grenoble Alpes, CEA, Grenoble INP, IRIG-PHELIQS, F-38000 Grenoble, France*

<sup>2</sup>*Laboratory for Muon-Spin Spectroscopy, Paul Scherrer Institute, CH-5232 Villigen-PSI, Switzerland*

<sup>3</sup>*Faculty of Physics, Babes-Bolyai University, 400084 Cluj-Napoca, Romania*

(Dated: December 22, 2023)

Details are provided on the derivation of the magnetic structure from the minimization of the energy, the computation of the polarization functions, and a comparison with a former model.

## S1. MINIMIZATION OF THE MAGNETIC ENERGY

We consider the nearest-neighbor Hamiltonian given in Eq. 1 with notations as defined in the main text.

There are twelve distinct bonds between nearest neighbors. They involve the position of Mn atoms in the origin and neighboring cubic unit cells. The lists of Mn sites and bonds are given in Tables S1 and S2. The different bonds are related to each other by symmetry operations of the point group associated with space group P2<sub>1</sub>3. The same operation links the Moriya vectors relative to each bond. Table S3 provides the relations between their Cartesian coordinates.

In the regular helical and conical structures the magnetic moment at Mn site  $\mathbf{i}$ ,  $\gamma$  is given by

$$\mathbf{m}_{\ell;\mathbf{i},\gamma} = m_{\perp} [\cos(\mathbf{k}_{\ell} \cdot \mathbf{r}_{\mathbf{i},\gamma}) \mathbf{a}_{\ell} - \sin(\mathbf{k}_{\ell} \cdot \mathbf{r}_{\mathbf{i},\gamma}) \mathbf{b}_{\ell}] + \mathbf{m}_{\parallel}, \quad (\text{S.1})$$

where  $\mathbf{a}_{\ell}$  and  $\mathbf{b}_{\ell}$  together with unit vector  $\hat{\mathbf{k}}_{\ell} = \mathbf{k}_{\ell}/k_{\ell}$  form a direct triad of unit vectors. Here we allow slight deviations from the regular structures:  $\mathbf{m}_{\ell;\mathbf{i},\gamma}$  obeys

TABLE S1. List of atoms involved in the considered bonds. For simplicity, we have dropped the subscript “Mn” in  $x_{\text{Mn}}$ . The superscripts ‘, ’’, and ’’’ denote translations  $-(1,0,0)$ ,  $-(0,1,0)$ , and  $-(0,0,1)$  relative to the original site.

| site   | coordinates               |
|--------|---------------------------|
| I      | $(x, x, x)$               |
| II     | $(1/2 - x, -x, x + 1/2)$  |
| II’    | $(-1/2 - x, -x, x + 1/2)$ |
| II’’   | $(1/2 - x, -x, x - 1/2)$  |
| III    | $(-x, x + 1/2, 1/2 - x)$  |
| III’’  | $(-x, x - 1/2, 1/2 - x)$  |
| III’’’ | $(-x, x + 1/2, -1/2 - x)$ |
| IV     | $(x + 1/2, 1/2 - x, -x)$  |
| IV’    | $(x - 1/2, 1/2 - x, -x)$  |
| IV’’   | $(x + 1/2, -1/2 - x, -x)$ |

TABLE S2. List of the twelve nearest-neighbor bonds considered in this work and symmetry operation of point group 23 linking each of them to the reference bond  $\mathbf{r}_{\text{I,II}}$ . The quantity  $R_a^{\theta}$  denotes a rotation of angle  $\theta$  about crystallographic axis  $a$ .

| bonds                            | coordinates             | symmetry operation                            |
|----------------------------------|-------------------------|-----------------------------------------------|
| $\mathbf{r}_{\text{I,II}}$       | $(1/2 - 2x, -2x, 1/2)$  | $= \mathbf{r}_{\text{I,II}}$                  |
| $\mathbf{r}_{\text{II’’’,I}}$    | $(2x - 1/2, 2x, 1/2)$   | $= R_{001}^{\pi} \mathbf{r}_{\text{I,II}}$    |
| $\mathbf{r}_{\text{I,III}}$      | $(-2x, 1/2, 1/2 - 2x)$  | $= R_{111}^{4\pi/3} \mathbf{r}_{\text{I,II}}$ |
| $\mathbf{r}_{\text{III’’’,I}}$   | $(2x, 1/2, 2x - 1/2)$   | $= R_{111}^{4\pi/3} \mathbf{r}_{\text{I,II}}$ |
| $\mathbf{r}_{\text{I,IV}}$       | $(1/2, 1/2 - 2x, -2x)$  | $= R_{111}^{2\pi/3} \mathbf{r}_{\text{I,II}}$ |
| $\mathbf{r}_{\text{IV’,I}}$      | $(1/2, 2x - 1/2, 2x)$   | $= R_{111}^{2\pi/3} \mathbf{r}_{\text{I,II}}$ |
| $\mathbf{r}_{\text{III’’,II’}}$  | $(-1/2, 1/2 - 2x, 2x)$  | $= R_{111}^{2\pi/3} \mathbf{r}_{\text{I,II}}$ |
| $\mathbf{r}_{\text{II,III’’}}$   | $(-1/2, 2x - 1/2, -2x)$ | $= R_{111}^{2\pi/3} \mathbf{r}_{\text{I,II}}$ |
| $\mathbf{r}_{\text{II’’’,IV’’}}$ | $(2x, -1/2, 1/2 - 2x)$  | $= R_{111}^{4\pi/3} \mathbf{r}_{\text{I,II}}$ |
| $\mathbf{r}_{\text{IV,II’’}}$    | $(-2x, -1/2, 2x - 1/2)$ | $= R_{111}^{4\pi/3} \mathbf{r}_{\text{I,II}}$ |
| $\mathbf{r}_{\text{IV’,III’’}}$  | $(1/2 - 2x, 2x, -1/2)$  | $= R_{100}^{\pi} \mathbf{r}_{\text{I,II}}$    |
| $\mathbf{r}_{\text{III,IV’}}$    | $(2x - 1/2, -2x, -1/2)$ | $= R_{010}^{\pi} \mathbf{r}_{\text{I,II}}$    |

TABLE S3. Expressions of the Moriya vectors as a function of the components of  $\mathbf{D}_{\text{I,II}}$  denoted as  $D^x$ ,  $D^y$ , and  $D^z$ .

| Moriya vector                    | symmetry operation                            | coordinates         |
|----------------------------------|-----------------------------------------------|---------------------|
| $\mathbf{D}_{\text{I,II}}$       | $= \mathbf{D}_{\text{I,II}}$                  | $(D^x, D^y, D^z)$   |
| $\mathbf{D}_{\text{II’’’,I}}$    | $= R_{001}^{\pi} \mathbf{D}_{\text{I,II}}$    | $(-D^x, -D^y, D^z)$ |
| $\mathbf{D}_{\text{I,III}}$      | $= R_{111}^{4\pi/3} \mathbf{D}_{\text{I,II}}$ | $(D^y, D^z, D^x)$   |
| $\mathbf{D}_{\text{III’’’,I}}$   | $= R_{111}^{4\pi/3} \mathbf{D}_{\text{I,II}}$ | $(-D^y, D^z, -D^x)$ |
| $\mathbf{D}_{\text{I,IV}}$       | $= R_{111}^{2\pi/3} \mathbf{D}_{\text{I,II}}$ | $(D^z, D^x, D^y)$   |
| $\mathbf{D}_{\text{IV’,I}}$      | $= R_{111}^{2\pi/3} \mathbf{D}_{\text{I,II}}$ | $(D^z, -D^x, -D^y)$ |
| $\mathbf{D}_{\text{III’’,II’}}$  | $= R_{111}^{2\pi/3} \mathbf{D}_{\text{I,II}}$ | $(-D^z, D^x, -D^y)$ |
| $\mathbf{D}_{\text{II,III’’}}$   | $= R_{111}^{2\pi/3} \mathbf{D}_{\text{I,II}}$ | $(-D^z, -D^x, D^y)$ |
| $\mathbf{D}_{\text{II’’’,IV’’}}$ | $= R_{111}^{4\pi/3} \mathbf{D}_{\text{I,II}}$ | $(-D^y, -D^z, D^x)$ |
| $\mathbf{D}_{\text{IV,II’’}}$    | $= R_{111}^{4\pi/3} \mathbf{D}_{\text{I,II}}$ | $(D^y, -D^z, -D^x)$ |
| $\mathbf{D}_{\text{IV’,III’’}}$  | $= R_{100}^{\pi} \mathbf{D}_{\text{I,II}}$    | $(D^x, -D^y, -D^z)$ |
| $\mathbf{D}_{\text{III,IV’}}$    | $= R_{010}^{\pi} \mathbf{D}_{\text{I,II}}$    | $(-D^x, D^y, -D^z)$ |

Eq. 4, in which  $\mathbf{a}_{\ell,\gamma}$  and  $\mathbf{b}_{\ell,\gamma}$  together with  $\mathbf{n}_{\ell,\gamma} = \mathbf{a}_{\ell,\gamma} \times \mathbf{b}_{\ell,\gamma}$  also form a direct triad of unit vectors. Now, a triad  $(\mathbf{n}_{\ell,1}, \mathbf{n}_{\ell,2}, \mathbf{n}_{\ell,3})$  is introduced, with  $\mathbf{n}_{\ell,3}$  close to  $\hat{\mathbf{k}}_{\ell}$ , in line with our assumption of magnetic structures closely related to the regular ones. Hereafter we will show that the energy is minimized for  $\mathbf{n}_{\ell,3} = \hat{\mathbf{k}}_{\ell}$ . In line with the incommensurate nature of the structure, the orientation of

$\mathbf{n}_{\ell,1}$  and  $\mathbf{n}_{\ell,2}$  in the plane perpendicular to  $\mathbf{k}$  can be arbitrarily chosen. Then, for simplicity, vectors  $\mathbf{n}_{\ell,1}$  and  $\mathbf{n}_{\ell,2}$  will be respectively identified to  $\mathbf{a}_\ell$  and  $\mathbf{b}_\ell$ . Back to triad  $(\mathbf{a}_{\ell,\gamma}, \mathbf{b}_{\ell,\gamma}, \mathbf{n}_{\ell,\gamma})$ , it is derived from  $(\mathbf{n}_{\ell,1}, \mathbf{n}_{\ell,2}, \mathbf{n}_{\ell,3})$  after two subsequent rotations. The first one corresponding to the structure twist is a rotation of angle  $\omega_{\ell,\gamma}$  around  $\mathbf{n}_{\ell,3}$ . The second one, defining the structure canting, is a rotation around an axis  $\mathbf{\Gamma}_{\ell,\gamma}$  perpendicular to  $\mathbf{n}_{\ell,3}$ , with an angle given by the modulus of  $\mathbf{\Gamma}_{\ell,\gamma}$ . Since there are four different  $\gamma$ 's, we have *a priori* a total of sixteen independent parameters: four  $\omega_{\ell,\gamma}$ 's and three Cartesian components of four  $\mathbf{\Gamma}_{\ell,\gamma}$  vectors [1].

We first consider the zero-field magnetic structure, setting  $\mathbf{m}_\parallel = 0$  in Eq. 4, and express the energy from Eq. 1. Recognizing the incommensurate nature of the structure and the fact that  $\mathbf{k}_\ell \cdot \mathbf{r}_{\mathbf{i},\gamma;\mathbf{i}',\gamma'}$ ,  $D/J$ ,  $\omega_{\ell,\gamma}$  and  $\mathbf{\Gamma}_{\ell,\gamma}$  are all much less than 1 in absolute value, this energy is expanded up to second order in these different quantities. Besides a constant, the result is a sum of two terms. With respect to the rotation angles, the former only depends on the four  $\omega_{\ell,\gamma}$  angles and the latter only on the components of  $\mathbf{\Gamma}_{\ell,\gamma}$  [2]. The minimization of each of the terms leads to  $\mathbf{n}_{\ell,3} = \hat{\mathbf{k}}_\ell$  and the following relations [2]:

$$\begin{aligned} \omega_{\ell,\text{II}} - \omega_{\ell,\text{I}} &= -2(k_\ell^x + k_\ell^y) \left( x - \frac{1}{8} \right) a_{\text{latt}} - \frac{\sigma}{2} (\hat{k}_\ell^x + \hat{k}_\ell^y), \\ \omega_{\ell,\text{III}} - \omega_{\ell,\text{I}} &= -2(k_\ell^x + k_\ell^z) \left( x - \frac{1}{8} \right) a_{\text{latt}} - \frac{\sigma}{2} (\hat{k}_\ell^x + \hat{k}_\ell^z), \\ \omega_{\ell,\text{IV}} - \omega_{\ell,\text{I}} &= -2 \left( k_\ell^y + k_\ell^z \right) \left( x - \frac{1}{8} \right) a_{\text{latt}} - \frac{\sigma}{2} (\hat{k}_\ell^y + \hat{k}_\ell^z), \\ \mathbf{\Gamma}_{\ell,\text{II}} - \mathbf{\Gamma}_{\ell,\text{I}} &= \frac{\sigma}{2} \left( \hat{k}_\ell^x \hat{k}_\ell^y - (\hat{k}_\ell^y)^2 - (\hat{k}_\ell^z)^2, \right. \\ &\quad \left. \hat{k}_\ell^x \hat{k}_\ell^y - (\hat{k}_\ell^x)^2 - (\hat{k}_\ell^z)^2, \hat{k}_\ell^x \hat{k}_\ell^z + \hat{k}_\ell^y \hat{k}_\ell^z \right), \\ \mathbf{\Gamma}_{\ell,\text{III}} - \mathbf{\Gamma}_{\ell,\text{I}} &= \frac{\sigma}{2} \left( \hat{k}_\ell^x \hat{k}_\ell^z - (\hat{k}_\ell^y)^2 - (\hat{k}_\ell^z)^2, \right. \\ &\quad \left. \hat{k}_\ell^x \hat{k}_\ell^y + \hat{k}_\ell^y \hat{k}_\ell^z, \hat{k}_\ell^x \hat{k}_\ell^z - (\hat{k}_\ell^x)^2 - (\hat{k}_\ell^y)^2 \right), \\ \mathbf{\Gamma}_{\ell,\text{IV}} - \mathbf{\Gamma}_{\ell,\text{I}} &= \frac{\sigma}{2} \left( \hat{k}_\ell^x \hat{k}_\ell^y + \hat{k}_\ell^x \hat{k}_\ell^z, \hat{k}_\ell^y \hat{k}_\ell^z - (\hat{k}_\ell^x)^2 - (\hat{k}_\ell^z)^2, \right. \\ &\quad \left. \hat{k}_\ell^y \hat{k}_\ell^z - (\hat{k}_\ell^x)^2 - (\hat{k}_\ell^y)^2 \right), \end{aligned} \quad (\text{S.2})$$

where  $\sigma$  is defined in Eq. 3 [3] and all the Cartesian components are expressed in the cubic reference frame. Moreover, it is found that the minimum of energy is independent of the direction of  $\mathbf{k}_\ell$ . With respect to  $k_\ell$ , the energy is minimum when Eq. 2 is satisfied [2].

Interestingly, only differences of angles appear in Eq. S.2. This is expected since in an incommensurate structure, the actual phase depends on the origin adopted for the reference frame. We are therefore authorized to enforce a new condition. We set  $\sum_\gamma \omega_{\ell,\gamma} = 0$ . Together with the first three lines of Eq. S.2, we have a set of four linear equations with four unknowns, which is readily solved. Similarly, we set  $\sum_\gamma \mathbf{\Gamma}_{\ell,\gamma} = 0$  and determine the four  $\mathbf{\Gamma}_{\ell,\gamma}$  vectors.

Inspecting Eq. S.2 it is remarkable that the twist and canting angles solely depend on parameter  $\sigma \equiv (D^x + D^y)/J$ , i.e. only the sum of two out of the three components of the Moriya vector matters. On the same footing,

the condition for minimizing the energy is given by Eq. 2, i.e. a linear combination of the three components of  $\mathbf{D}$ . As a matter of fact, the model is not dependent on each of the  $\mathbf{D}$  components, but only on two linear combinations of them.

We turn to the case of the conical phase. The energy is computed from Eqs. 1 and 4, in the same way as in the helical phase, except that  $m_\parallel$  is a free parameter. The minimization leads to results similar to those obtained in the helical phase [2]. The cone angle  $\theta$  is found to be proportional to  $B$  with

$$\cos \theta = \frac{m_\parallel}{m} = \frac{6Jg\mu_B B}{(-D^x + D^y - 2D^z)^2}. \quad (\text{S.3})$$

Although Eq. S.3 links  $m_\perp$  and  $m_\parallel$ , thanks to the very high sensitivity of  $\mu\text{SR}$  to these quantities, the fit presented in Fig. 1 was performed leaving them as free parameters for each of the spectra recorded under a magnetic field. We note that the application of Eq. S.3 using the numerical values presented in the main text leads to  $\theta = 59(3)$  degrees, in fair agreement with the values reported in Table II.

At this juncture we notice that the helical and conical structures are fully determined by the linear combination of ratios  $D^\alpha/J$  appearing in Eqs. 2 and 3. The cone angle of the conical structure does not provide an additional combination.

With the determination of the rotation parameters we can fully determine vectors  $\mathbf{a}_{\ell,\gamma}$  and  $\mathbf{b}_{\ell,\gamma}$  of Eq. 4, and therefore the magnetic structure. With this material at hand we can proceed to the computation of the  $\mu\text{SR}$  polarization functions.

## S2. THE $P_Z(t)$ AND $P_X(t)$ POLARIZATION FUNCTIONS

The relevant  $\mu\text{SR}$  signals are measured in pairs of detectors BF and UD in zero-field and UD and LR in an applied field, with a notation explicated in Fig. 1. Polarization function  $P_Z(t)$  is relevant in zero-field for both BF and UD pairs of detectors. In finite field, the signal measured in the pair UD is  $P_X(t)$  and that measured in the pair LR is  $P_Y(t)$ . The Cartesian axes  $X$ ,  $Y$ , and  $Z$  refer to a laboratory orthogonal reference frame. The muon beam polarization defines the  $Z$  axis for zero-field measurements, while this  $Z$  axis is collinear to  $\mathbf{B}_{\text{ext}}$  for experiments performed in an applied field [4, 5].

This section is devoted to the derivation of the  $P_Z(t)$  and  $P_X(t)$  polarization functions. The methodology followed for the derivation of  $P_Y(t)$  is very similar to that of  $P_X(t)$ : the interested reader will adapt the  $P_X(t)$  formulas to  $P_Y(t)$ .

As will be seen, the expression of the polarization functions require the Fourier components of the magnetic moments in the crystal. We first explicit their expression and turn to the evaluation of  $P_Z(t)$  and  $P_X(t)$  in a second step.

### A. Fourier components $\mathbf{m}_{\ell;\mathbf{q},\gamma}$

With the Fourier transformation definition,

$$\mathbf{m}_{\ell;\mathbf{q},\gamma} = \frac{1}{\sqrt{n_c}} \sum_{\mathbf{i}} \mathbf{m}_{\ell;\mathbf{i},\gamma} \exp[-i\mathbf{q} \cdot (\mathbf{i} + \mathbf{d}_\gamma)], \quad (\text{S.4})$$

where the sum runs over the coordinates  $\mathbf{i}$  of the  $n_c$  cubic unit cells of the crystal and  $\mathbf{q}$  is a vector of the first Brillouin zone. Equations 4 and S.4 lead to

$$\mathbf{m}_{\ell;\mathbf{q},\gamma} = \sqrt{n_c} (\delta_{\mathbf{q},\mathbf{k}} \tilde{\mathbf{m}}_{\ell;\gamma,+} + \delta_{\mathbf{q},-\mathbf{k}} \tilde{\mathbf{m}}_{\ell;\gamma,-} + \delta_{\mathbf{q},\mathbf{0}} \mathbf{m}_{\parallel}), \quad (\text{S.5})$$

with

$$\tilde{\mathbf{m}}_{\ell;\gamma,\pm} = \frac{m_{\perp}}{2} (\mathbf{a}_{\ell,\gamma} \pm i\mathbf{b}_{\ell,\gamma}). \quad (\text{S.6})$$

### B. Derivation of $P_Z(t)$ and $P_X(t)$

The polarization functions denoted as  $P_Z(t)$  and  $P_X(t)$  are respectively measured for the zero and finite field  $\mu\text{SR}$  experiments. These are the average evolutions of the  $Z$  and  $X$  components of the spin  $\mathbf{S}_\mu$  of the muons implanted into the specimen under study. We start with the motion of a muon spin submitted to field  $\mathbf{B}_{\text{loc}}$ . It is ruled by the Larmor equation whose solution reads

$$\frac{S_Z(t)}{S} = \left(\frac{B^Z}{B}\right)^2 + \left[1 - \left(\frac{B^Z}{B}\right)^2\right] \cos(\gamma_\mu B t), \quad (\text{S.7})$$

and

$$\begin{aligned} S_X(t)/S = & \left\{ \frac{B_X^2}{B^2} + \left(1 - \frac{B_X^2}{B^2}\right) \cos(\omega_\mu t) \right\} \cos \varphi_\mu \sin \theta_\mu \\ & + \left\{ \frac{B_X B_Y}{B^2} [1 - \cos(\omega_\mu t)] + \frac{B_Z}{B} \sin(\omega_\mu t) \right\} \sin \varphi_\mu \sin \theta_\mu \\ & + \left\{ \frac{B_X B_Z}{B^2} [1 - \cos(\omega_\mu t)] - \frac{B_Y}{B} \sin(\omega_\mu t) \right\} \cos \theta_\mu, \quad (\text{S.8}) \end{aligned}$$

respectively for  $S_Z(t)$  and  $S_X(t)$  [6]. For simplicity and since there is no risk of confusion in this section, we have dropped the subscript  $\mu$  of  $\mathbf{S}_\mu$  and “loc” of  $\mathbf{B}_{\text{loc}}$ . In Eq. S.8,  $\mathbf{S}$  is assumed to be oriented at time 0 in the direction defined by the polar and azimuthal angles  $\theta_\mu$  and  $\varphi_\mu$ , corresponding to the experimental conditions. We do not worry about the direction of the muon spin at the instant of implantation in Eq. S.7, since the zero-field  $P_Z(t)$  is independent of this direction [7]. For definiteness, Eq. S.7 is derived for a muon spin oriented along the  $Z$  axis at time 0.

We turn to the expression of the field at the muon site. This field is the sum of the applied field  $\mathbf{B}_{\text{ext}}$  and the field resulting from the Mn magnetic moments. The latter is decomposed in three parts: the first one stems

from the moments in the Lorentz sphere, the second is the Lorentz field  $\mathbf{B}_{\text{Lor}}$ , and the third is the demagnetization field  $\mathbf{B}_{\text{dem}}$ .

The field arising from the moments in the Lorentz sphere depends on the position of the muon in the crystal unit cell, the Mn magnetic moments and their coupling with the probe. In a metal this coupling is traditionally split into two contributions, (i) the classical dipolar interaction with the Mn electronic moments assumed to be localized at the Mn position, and (ii) the Fermi contact interaction of the muon spin with the electron density at its site, which is polarized by the neighboring Mn magnetic moments. Both contributions linearly depend on the magnetic moments  $\mathbf{m}_{\ell;\mathbf{i},\gamma}$ . Because of the long-range nature of the magnetic structure, it is advantageous to use the Ewald transformation for the computation of the dipolar contribution [8, 9]. Therefore we represent the magnetic moments in the lattice by their Fourier transform. Altogether the field at muon site  $s_\eta$  in K-domain  $\ell$  is

$$\begin{aligned} \mathbf{B}_{\text{loc},\ell,s_\eta} = & \mathbf{B}_{\text{ext}} + \mathbf{B}_{\text{Lor}} + \mathbf{B}_{\text{dem}} \\ & + \frac{\mu_0}{4\pi} \frac{1}{\sqrt{n_c} v_c} \sum_{\gamma} \sum_{\mathbf{q}} \mathbf{G}_{d_\gamma,\mathbf{q},s_\eta} \mathbf{m}_{\ell,d_\gamma,\mathbf{q}} \exp(-i\mathbf{q} \cdot \mathbf{r}_{0,s_\eta}). \end{aligned} \quad (\text{S.9})$$

Here,  $v_c$  is the volume of the unit cubic cell. Tensor  $\mathbf{G}_{d_\gamma,\mathbf{q},s_\eta}$  describes the dipolar and Fermi contact interactions between the muon spin and the Mn magnetic moments; see Refs. 5, 7, and 10 for full details. The Fermi contact interaction is characterized by the unitless parameter  $r_\mu H/4\pi = -1.04(1)$  [7, 11, 12]. Parameter  $-\mathbf{r}_{0,s_\eta}$  in Eq. S.9 is the vector position of the muon in the crystal unit cell. Experiments dedicated to the determination of the muon site in MnSi showed the muon to be located at an interstitial site corresponding to Wyckoff position  $4a$  of space group  $P2_13$ , of coordinate  $(x_\mu, x_\mu, x_\mu)$  with  $x_\mu = 0.532$  in reduced unit [11]. There are therefore four possible sites, labelled by  $s_\eta$ , for the muon in the cubic cell.

Fields  $\mathbf{B}_{\text{Lor}}$  and  $\mathbf{B}_{\text{dem}}$  are respectively equal to  $4\mu_0 \mathbf{m}_{\parallel}/3v_c$  and  $-4\mu_0 N \mathbf{m}_{\parallel}/v_c$ . The factor 4 accounts for the four Mn atoms in the unit cubic cell and  $N \approx 0.8$  is the demagnetizing field coefficient.

The next step towards the expression of  $P_{Z,X}(t)$  is to include the effect of spin-lattice and spin-spin relaxations in the model. This is achieved by multiplying the non-oscillating contribution of  $S_Z(t)$  by  $\exp(-\lambda_Z t)$  and the oscillating contributions of  $S_Z(t)$  and  $S_X(t)$  by  $\exp(-\lambda_X t)$  (Eqs. S.7 and S.8). Here,  $\lambda_Z$  and  $\lambda_X$  are respectively the spin-lattice and spin-spin relaxation rates, but in the fitting procedure  $\lambda_X$  may also phenomenologically include the effect of a possible small disorder in the crystal or magnetic structure.

In a  $\mu\text{SR}$  measurement several millions of muons are implanted in the specimen under study. Each of them localizes in a random unit cell of the crystal. Therefore parameter  $-\mathbf{r}_{0,s_\eta}$  of Eq. S.9 takes many possible values which differ by a vector equal to a lattice Bravais vector.

Recalling that the magnetic structure is incommensurate, this implies that factor  $\exp(-i\mathbf{q} \cdot \mathbf{r}_{0,s_\eta})$  for  $\mathbf{q} = \pm\mathbf{k}$  in Eq. S.9 uniformly spans the unit circle in the complex plane. The ensemble of implanted muons therefore probe a distribution of fields, denoted as  $D_v(\mathbf{B})$ , rather than  $\mathbf{B}_{\text{loc},\ell,s_\eta}$  [7]. Then, the polarization functions associated with muons implanted at site  $s_\eta$  in domain  $\ell$  write

$$P_{Z,X,\ell,s_\eta}(t) = \int \frac{S_{Z,X}(t)}{S} D_v(\mathbf{B}) d^3\mathbf{B}, \quad (\text{S.10})$$

and the average over the four muon sites and the four K-domains is

$$P_{Z,X}(t) = \langle P_{Z,X,\ell,s_\eta}(t) \rangle_{\ell,\eta}. \quad (\text{S.11})$$

Finally the actual fit function is obtained by including the signal arising from the fraction  $f$  of muons which miss the sample and stop in its surroundings, i.e.

$$P_{Z,X}^{\text{fit}}(t) = (1-f)P_{Z,X}(t) + f \cos(\omega_{\text{ext}}t - \varphi_\mu). \quad (\text{S.12})$$

Fraction  $f$  is 0 for the [111] crystal owing to its very large cross section and  $f \lesssim 0.04$  for the other two crystals. In addition,  $\omega_{\text{ext}} \approx \gamma_\mu B_{\text{ext}}$ .

### S3. COMPARISON WITH A FORMER MODEL FOR THE MAGNETIC STRUCTURE

The  $\mu\text{SR}$  spectra recorded in the helical and conical phases of MnSi presented in Refs. 7 and 13 as well as those of the present work cannot be modelled within the regular magnetic structures. In the cited references, deviations from these structures were allowed with limitations enforced by the symmetry of the  $P2_13$  space group and

the direction of the magnetic propagation wavevector in the crystal structure. This was technically achieved with the theory of representation analysis [14]. Restricting to structures close the regular structures, the deviations can be interpreted into twists and cantings acting in different ways on the four Mn sublattices and depending on the direction of the propagation wavevector. Now, representation analysis provides relation neither between the twist and canting angles nor between the angles observed for the different orientations of  $\mathbf{k}$ . Therefore a large number of unrelated parameters remain in the fitting procedure.

In the present work we use a model based on a microscopic Hamiltonian, with a full account of the crystal structure. It is assumed that the magnetic structure can be twisted and canted with, in a first step, no restriction on the twist and canting angles and in particular with the direction of canting. From the minimization of the magnetic energy the twist and canting angles are determined as a function of the physical parameters of the Hamiltonian. The resulting twisted and canted magnetic structure is fully consistent with representation analysis, notably the direction of canting which is severely constrained by symmetry. This is actually not surprising since the lattice symmetry is embedded in the origin Hamiltonian. The fit to the experimental spectra recorded in zero and finite fields applied along the three principal directions is then performed with a very limited number of parameters, which are physical parameters entering the Hamiltonian.

If we compare the polarization functions resulting from fits of the current model and those of Refs. [7, 13], the differences are tiny. For instance, considering the zero-field data, the most notable evolution in the field distributions is a separation between the two peaks located below 100 mT which is slightly smaller in the new model.

- 
- [1] The relation between quantities  $\omega_{\ell,\gamma}$  and  $\omega_{\ell',\gamma}$  in the one hand and  $\Gamma_{\ell,\gamma}$  and  $\Gamma_{\ell',\gamma}$  in the other hand are given by the symmetry operations related the corresponding K-domains  $\ell$  and  $\ell'$ .
  - [2] V. A. Chizhikov and V. E. Dmitrienko, Frustrated magnetic helices in MnSi-type crystals, *Phys. Rev. B* **85**, 014421 (2012).
  - [3] The mathematical expressions given in Eqs. 2, 3, and S.2 slightly differ from those of Ref. 2. There are two reasons for this. (i) The reference bond we adopt is between Mn sites I and II rather than I and III in Ref. 2. (ii) We consider here a left-handed helix as implicit from Eq. 4. This corresponds to a negative  $k$  parameter in the notation of Ref. 2.
  - [4] P. Dalmas de Réotier and A. Yaouanc, Muon spin rotation and relaxation in magnetic materials, *J. Phys.: Condens. Matter* **9**, 9113 (1997).
  - [5] A. Yaouanc and P. Dalmas de Réotier, *Muon Spin Rotation, Relaxation, and Resonance: Applications to Condensed Matter* (Oxford University Press, Oxford, 2011).

- [6] See, e.g., Eqs 3.10-13 of Ref. 5.
- [7] P. Dalmas de Réotier, A. Maisuradze, A. Yaouanc, B. Roessli, A. Amato, D. Andreica, and G. Lapertot, Determination of the zero-field magnetic structure of the helimagnet MnSi at low temperature, *Phys. Rev. B* **93**, 144419 (2016).
- [8] P. P. Ewald, Die Berechnung optischer und elektrostatischer Gitterpotentiale, *Ann. Phys.* **369**, 253 (1921).
- [9] M. Born and K. Huang, *Dynamical theory of crystal lattices* (Clarendon, Oxford, 1954).
- [10] A. Yaouanc, P. Dalmas de Réotier, and E. Frey, Zero-field muon-spin-relaxation depolarization rate of paramagnets near the Curie temperature, *Phys. Rev. B* **47**, 796 (1993).
- [11] A. Amato, P. Dalmas de Réotier, D. Andreica, A. Yaouanc, A. Suter, G. Lapertot, I. M. Pop, E. Morenzoni, P. Bonfà, F. Bernardini, and R. de Renzi, Understanding the  $\mu\text{SR}$  spectra of MnSi without magnetic polarons, *Phys. Rev. B* **89**, 184425 (2014).
- [12] P. Dalmas de Réotier, A. Yaouanc, A. Amato, A. Maisuradze, D. Andreica, B. Roessli, T. Goko,

- R. Scheuermann, and G. Lapertot, On the robustness of the MnSi magnetic structure determined by muon spin rotation, *Quantum Beam Sci.* **2**, 19 (2018).
- [13] P. Dalmas de Réotier, A. Maisuradze, A. Yaouanc, B. Roessli, A. Amato, D. Andreica, and G. Lapertot, Unconventional magnetic order in the conical state of MnSi, *Phys. Rev. B* **95**, 180403(R) (2017).
- [14] E. F. Bertaut, in *Treatise on Magnetism*, Vol. III, edited by H. Suhl and G. T. Rado (Academic Press, New York, 1963) Chap. 4; Representation analysis of magnetic structures, *Acta Crystallogr A* **24**, 217 (1968); Magnetic structure analysis and group theory, *J. Phys. Colloques* **32**, C1:462 (1971); On group theoretical techniques in magnetic structure analysis, *J. Magn. Magn. Mater.* **24**, 267 (1981).
